# Supplementary material for: A complementary screening for quantum spin Hall insulators in 2D exfoliable materials
Source: arXiv:2205.02583 source file (2023-09-15)
Supplement: Supplementary file 1 [file suppl.pdf]

# Supplemental Material: A complementary screening for quantum spin Hall insulators in 2D exfoliable materials

Davide Grassano,[1,*] Davide Campi,[1,2] Antimo Marrazzo,[1,3] and Nicola Marzari[1]

[1] *Theory and Simulations of Materials (THEOS) and National Center for Computational Design and Discovery of Novel Materials (MARVEL), École Polytechnique Fédérale de Lausanne, CH-1015 Lausanne, Switzerland*

[2] *Dipartimento di Scienza dei Materiali, Universita di Milano-Bicocca, Via Cozzi 53, 20125 Milano, Italy*

[3] *Dipartimento di Fisica, Università di Trieste, I-34151 Trieste, Italy*

Quantum spin Hall insulators are a class of topological materials that has been extensively studied during the past decade. One of their distinctive features is the presence of a finite band gap in the bulk and gapless, topologically protected edge states that are spin-momentum locked. These materials are characterized by a $\mathbb{Z}_2$ topological order where, in the 2D case, a single topological invariant can be even or odd for a trivial or a topological material, respectively. Thanks to their interesting properties, such as the realization of dissipationless spin currents, spin pumping and spin filtering, they are of great interest in the field of electronics, spintronics and quantum computing. In this paper we perform an high-throughput screening of quantum spin Hall insulators starting from a set of 783 two-dimensional exfoliable materials, recently identified from a systematic screening of the ICSD, COD, and MPDS databases. We find a new $\mathbb{Z}_2$ topological insulator ($Hg_4N_4S_4$) as well as 3 already known ones and 7 direct gap metals that have the potential of becoming quantum spin Hall insulators under a reasonable external perturbation.

## I. CONTENT

Here we present a collection of the data for every material determined to be either a quantum spin Hall insulator or a direct gap metal. For each, we report a table of the structural parameters, including the direct lattice vectors and the positions of the atoms in the relaxed structure. We also show the band structure, both with and without SOC, and, for non inversion-symmetric materials we also show the plot of the HWCC evolution. Finally, for every material we also show a bird-eye view of its crystal structure rendered using VESTA[1].

## II. QSHI

### A. $Br_2Hf_2$

| | |
|---|---|
| **Formula**: | $Br_2Hf_2$ |
| **Database ID**: | MPDS S546529 |
| **3D Spacegroup**: | 166 (R$\bar{3}$m) |
| **Inversion symmetry**: | YES |
| **Direct Gap [meV]**: | 232.8 |
| **Indirect gap [meV]**: | 48.3 |
| **Binding energy DF2-C09 [meV/Å$^2$]**: | 15.8 |

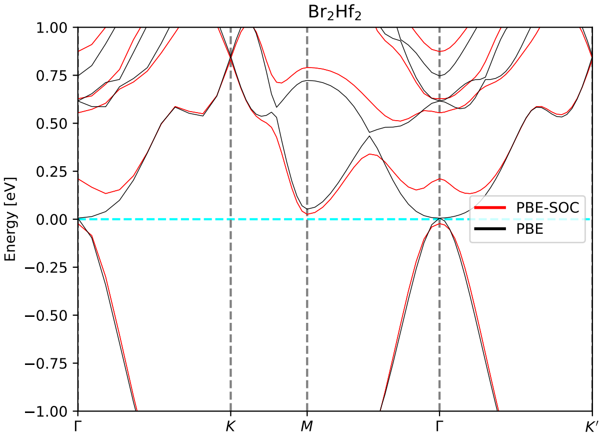


FIG. 1: DFT band structure with (red) and without (black) spin-orbit coupling.

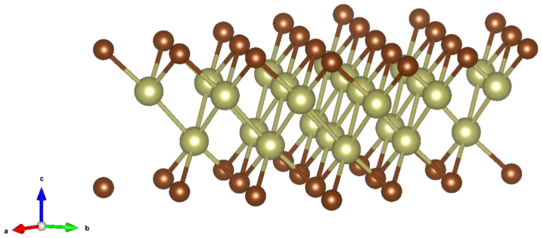

FIG. 2: Bird-eye view of the crystal structure.

TABLE I: Structural parameters

| | X[Å] | Y[Å] | Z[Å] |
|---|---|---|---|
| **a1** | 1.7402 | -3.0141 | 0.0000 |
| **a2** | 1.7402 | 3.0141 | 0.0000 |
| **a3** | 0.0000 | 0.0000 | 24.0847 |
| Hf | 1.7402 | 1.0047 | -1.1321 |
| Br | 0.0000 | 0.0000 | -3.0392 |
| Hf | 1.7402 | -1.0047 | 1.1321 |
| Br | 0.0000 | 0.0000 | 3.0392 |

### B. $Hf_2Te_{10}$

| | |
|---|---|
| **Formula**: | $Hf_2Te_{10}$ |
| **Database ID**: | MPDS S455329 |
| **3D Spacegroup**: | 63 (Cmcm) |
| **Inversion symmetry**: | NO |
| **Direct Gap [meV]**: | 299.3 |
| **Indirect gap [meV]**: | 171.0 |
| **Binding energy DF2-C09 [meV/Å$^2$]**: | 16.5 |

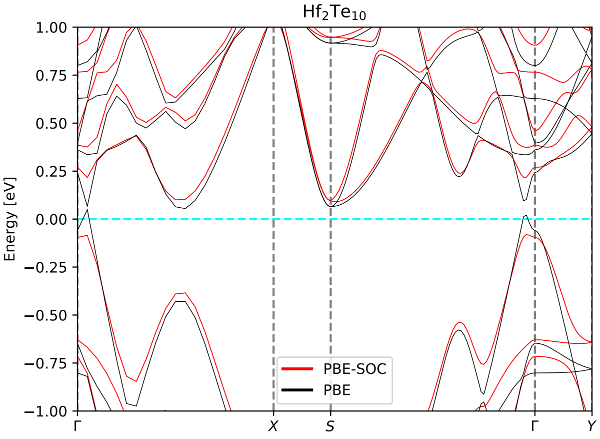


FIG. 3: DFT band structure with (red) and without (black) spin-orbit coupling.

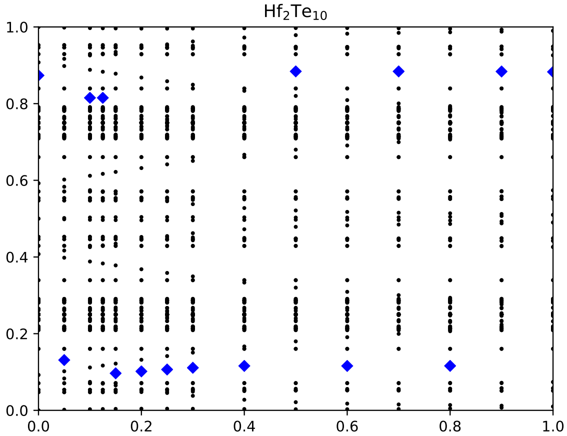


FIG. 4: Evolution of the HWCC (black dots) and largest gap positions (blue squares) across the Brillouin zone.

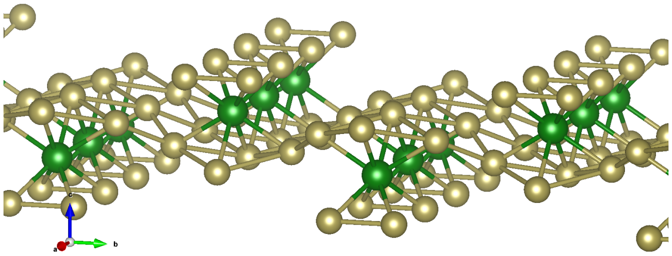

FIG. 5: Bird-eye view of the crystal structure.

TABLE II: Structural parameters

| | X[Å] | Y[Å] | Z[Å] |
|---|---|---|---|
| **a1** | 4.0291 | 0.0000 | 0.0000 |
| **a2** | 0.0000 | 13.8324 | 0.0000 |
| **a3** | 0.0000 | 0.0000 | 22.3851 |
| Hf | -1.0073 | -17.2905 | -0.9906 |
| Hf | 1.0073 | -10.3743 | 0.9906 |
| Te | 1.0073 | -17.2905 | 1.2315 |
| Te | -1.0073 | -10.3743 | -1.2315 |
| Te | -1.0073 | -19.8333 | 0.5747 |
| Te | 1.0073 | -12.9171 | -0.5747 |
| Te | 1.0073 | -7.8316 | -0.5747 |
| Te | -1.0073 | -14.7478 | 0.5747 |
| Te | 1.0073 | -15.8953 | -2.6504 |
| Te | -1.0073 | -8.9790 | 2.6504 |
| Te | -1.0073 | -11.7696 | 2.6504 |
| Te | 1.0073 | -18.6858 | -2.6504 |

### C. $Hg_4N_4S_4$

| | |
|---|---|
| **Formula**: | $Hg_4N_4S_4$ |
| **Database ID**: | MPDS S1703098 |
| **3D Spacegroup**: | 61 (Pbca) |
| **Inversion symmetry**: | NO |
| **Direct Gap [meV]**: | 7.1 |
| **Indirect gap [meV]**: | 7.1 |
| **Binding energy DF2-C09 [meV/Å$^2$]**: | 19.4 |

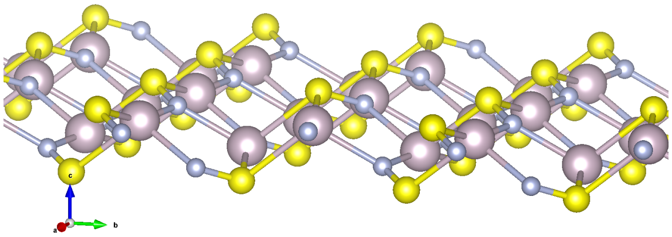

FIG. 8: Bird-eye view of the crystal structure.

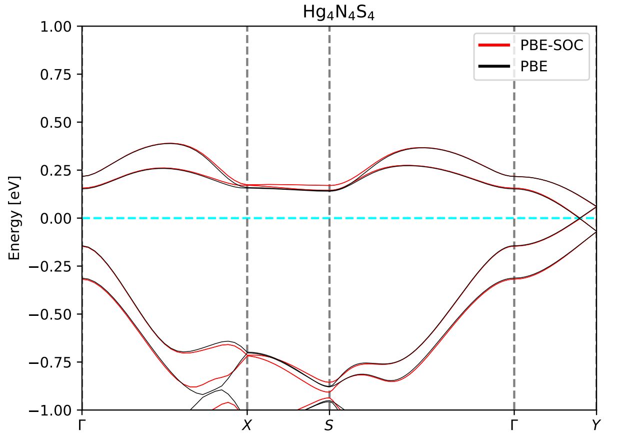


FIG. 6: DFT band structure with (red) and without (black) spin-orbit coupling.

TABLE III: Structural parameters

| | X[Å] | Y[Å] | Z[Å] |
|---|---|---|---|
| **a1** | 5.3686 | -0.0018 | 0.0000 |
| **a2** | -0.0201 | 10.7795 | 0.0000 |
| **a3** | 0.0000 | 0.0000 | 16.9180 |
| Hg | -6.4161 | 1.4264 | 0.5240 |
| Hg | -3.7342 | 3.9802 | -0.5538 |
| Hg | -4.3412 | 9.3567 | -0.5240 |
| Hg | -7.0231 | 6.8029 | 0.5538 |
| S | -6.6170 | -0.8389 | -1.2004 |
| S | -3.9513 | 6.2104 | 1.2206 |
| S | -4.1202 | 0.8425 | 1.2004 |
| S | -6.8060 | 4.5727 | -1.2206 |
| N | -7.6635 | 8.8272 | -0.6895 |
| N | -4.9765 | 7.3325 | 0.7252 |
| N | -3.0938 | 1.9559 | 0.6895 |
| N | -5.7808 | 3.4506 | -0.7252 |

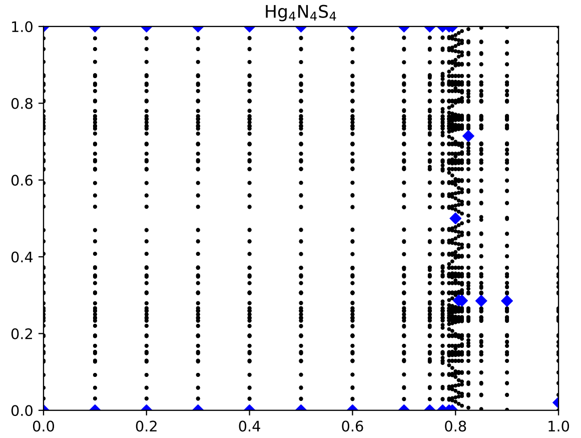


FIG. 7: Evolution of the HWCC (black dots) and largest gap positions (blue squares) across the Brillouin zone.

### D. $Te_{10}Zr_2$

| | |
|---|---|
| **Formula**: | $Te_{10}Zr_2$ |
| **Database ID**: | MPDS S457010 |
| **3D Spacegroup**: | 63 (Cmcm) |
| **Inversion symmetry**: | NO |
| **Direct Gap [meV]**: | 280.7 |
| **Indirect gap [meV]**: | 219.6 |
| **Binding energy DF2-C09 [meV/Å$^2$]**: | 19.4 |

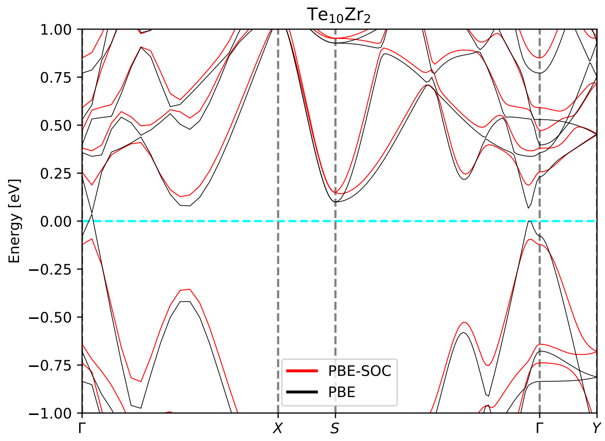


FIG. 9: DFT band structure with (red) and without (black) spin-orbit coupling.

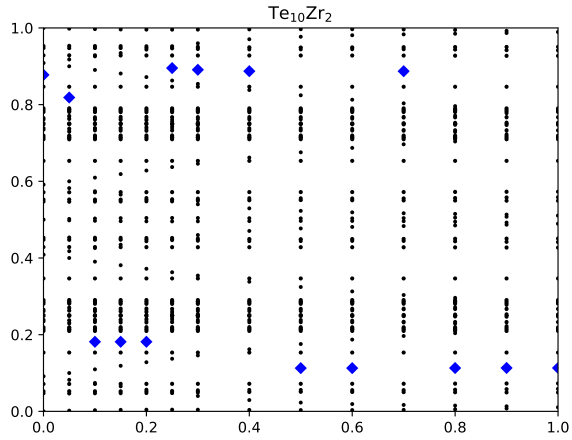


FIG. 10: Evolution of the HWCC (black dots) and largest gap positions (blue squares) across the Brillouin zone.

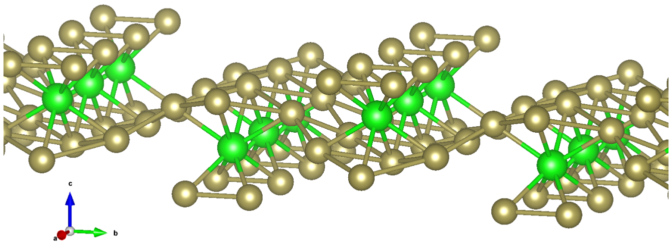

FIG. 11: Bird-eye view of the crystal structure.

TABLE IV: Structural parameters

| | X[Å] | Y[Å] | Z[Å] |
|---|---|---|---|
| **a1** | 4.0472 | 0.0000 | 0.0000 |
| **a2** | 0.0000 | 13.8438 | 0.0000 |
| **a3** | 0.0000 | 0.0000 | 22.4715 |
| Zr | 1.0118 | -10.3829 | -1.0016 |
| Zr | -1.0118 | -3.4610 | 1.0016 |
| Te | -1.0118 | -11.7748 | -2.6768 |
| Te | 1.0118 | -2.0690 | 2.6768 |
| Te | -1.0118 | -8.9910 | -2.6768 |
| Te | 1.0118 | -4.8529 | 2.6768 |
| Te | -1.0118 | -10.3829 | 1.2327 |
| Te | 1.0118 | -3.4610 | -1.2327 |
| Te | 1.0118 | -7.8333 | 0.5745 |
| Te | -1.0118 | -6.0105 | -0.5745 |
| Te | 1.0118 | -12.9324 | 0.5745 |
| Te | -1.0118 | -0.9114 | -0.5745 |

## III. DGM

### A. $BaCr_2N_2O_8$

| | |
|---|---|
| **Formula**: | $BaCr_2N_2O_8$ |
| **Database ID**: | MPDS S1704934 |
| **3D Spacegroup**: | 166 (R$\bar{3}$m) |
| **Inversion symmetry**: | YES |
| **Direct Gap [meV]**: | 19.3 |
| **Indirect gap [meV]**: | -124.0 |
| **Binding energy DF2-C09 [meV/Å$^2$]**: | 11.0 |

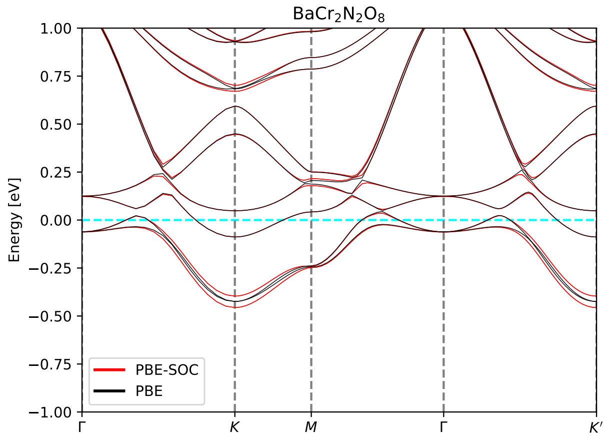


FIG. 12: DFT band structure with (red) and without (black) spin-orbit coupling.

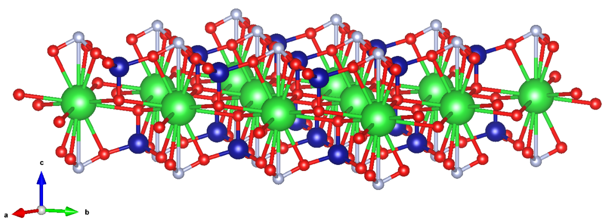

FIG. 13: Bird-eye view of the crystal structure.

TABLE V: Structural parameters

| | X[Å] | Y[Å] | Z[Å] |
|---|---|---|---|
| **a1** | 2.6064 | -4.5145 | 0.0000 |
| **a2** | 2.6064 | 4.5145 | 0.0000 |
| **a3** | 0.0000 | 0.0000 | 24.7486 |
| Cr | 3.9097 | -0.7524 | 2.1565 |
| N | 1.3032 | -2.2572 | 3.2679 |
| O | 2.4168 | -1.6143 | 2.6330 |
| O | 1.3032 | -3.5431 | 2.6330 |
| O | 0.1897 | -1.6143 | 2.6330 |
| O | 1.3032 | 0.7524 | -0.4977 |
| Cr | 1.3032 | 0.7524 | -2.1565 |
| N | 1.3032 | -2.2572 | -3.2679 |
| O | 2.4168 | -2.9002 | -2.6330 |
| O | 1.3032 | -0.9714 | -2.6330 |
| O | 0.1897 | -2.9002 | -2.6330 |
| O | 3.9097 | -0.7524 | 0.4977 |
| Ba | 1.3032 | -2.2572 | 0.0000 |

### B. $Br_6V_2$

| | |
|---|---|
| **Formula**: | $Br_6V_2$ |
| **Database ID**: | MPDS S1902638 |
| **3D Spacegroup**: | 148 ($R\bar{3}$) |
| **Inversion symmetry**: | YES |
| **Direct Gap [meV]**: | 32.9 |
| **Indirect gap [meV]**: | -99.4 |
| **Binding energy DF2-C09 [meV/Å$^2$]**: | 15.1 |

TABLE VI: Structural parameters

| | X[Å] | Y[Å] | Z[Å] |
|---|---|---|---|
| **a1** | 3.1108 | 5.3881 | 0.0000 |
| **a2** | -3.1108 | 5.3881 | 0.0000 |
| **a3** | 0.0000 | 0.0000 | 17.9200 |
| V | 0.0000 | -3.5920 | 0.0000 |
| V | -3.1108 | -1.7960 | 0.0000 |
| Br | -4.1801 | -3.5359 | -1.4813 |
| Br | -2.1386 | 0.0000 | 1.4813 |
| Br | -2.0415 | -3.5359 | 1.4813 |
| Br | -5.1523 | -1.8521 | 1.4813 |
| Br | -4.0830 | 0.0000 | -1.4813 |
| Br | -1.0693 | -1.8521 | -1.4813 |

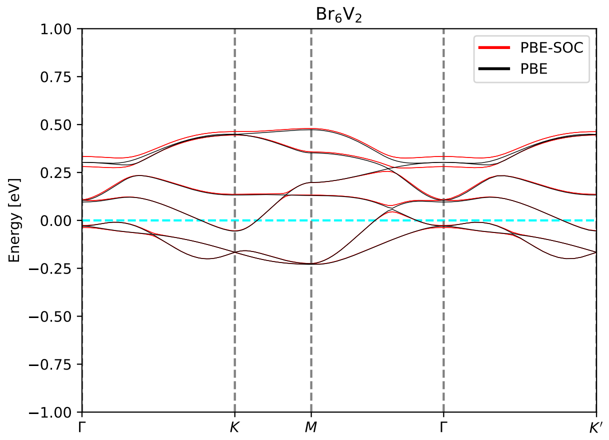


FIG. 14: DFT band structure with (red) and without (black) spin-orbit coupling.

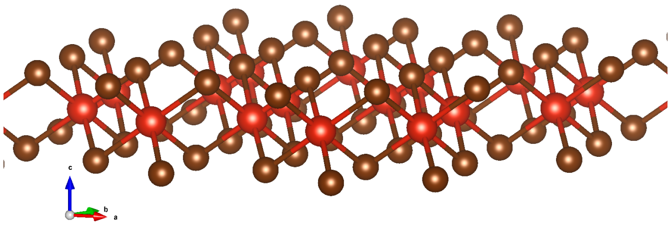

FIG. 15: Bird-eye view of the crystal structure.

### C. $C_2H_6Fe_2O_8P_2$

| | |
|---|---|
| **Formula**: | $C_2H_6Fe_2O_8P_2$ |
| **Database ID**: | MPDS S1125577 |
| **3D Spacegroup**: | 2 ($P\bar{1}$) |
| **Inversion symmetry**: | NO |
| **Direct Gap [meV]**: | 10.7 |
| **Indirect gap [meV]**: | -58.4 |
| **Binding energy DF2-C09 [meV/Å$^2$]**: | 18.8 |

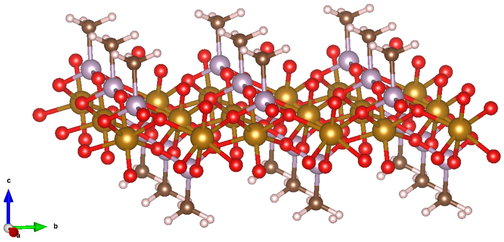

FIG. 18: Bird-eye view of the crystal structure.

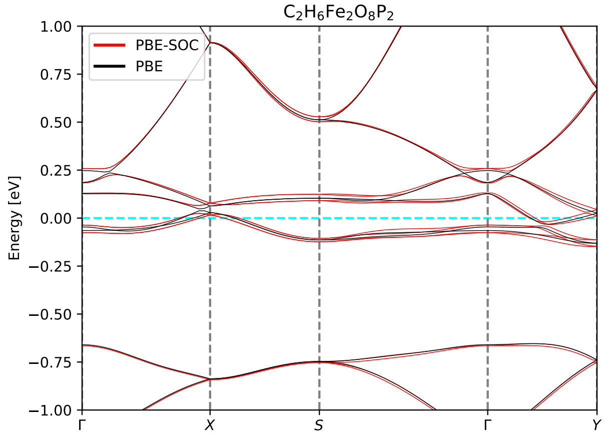


FIG. 16: DFT band structure with (red) and without (black) spin-orbit coupling.

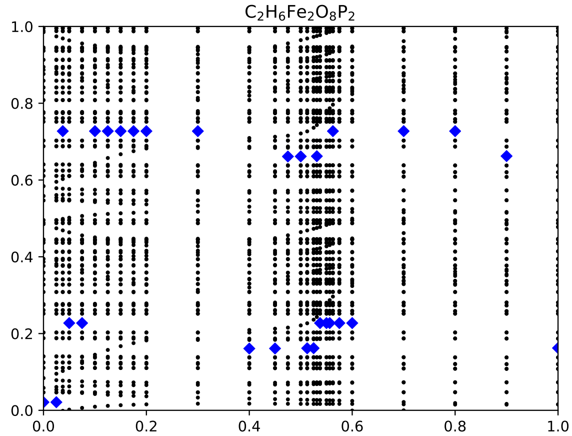


FIG. 17: Evolution of the HWCC (black dots) and largest gap positions (blue squares) across the Brillouin zone.

TABLE VII: Structural parameters

| | X[Å] | Y[Å] | Z[Å] |
|---|---|---|---|
| **a1** | 4.7069 | 0.0001 | 0.0000 |
| **a2** | 0.0001 | 5.5134 | 0.0000 |
| **a3** | 0.0000 | 0.0000 | 27.1570 |
| Fe | 1.7832 | 1.0894 | -0.1656 |
| Fe | 4.1367 | 3.8461 | 0.1656 |
| P | 1.4160 | 3.8460 | -1.5644 |
| P | 3.7694 | 1.0894 | 1.5644 |
| H | 1.3837 | 4.7506 | -3.7631 |
| H | 3.7371 | 1.9939 | 3.7631 |
| H | 4.5854 | 3.8392 | -3.3781 |
| H | 2.2320 | 1.0825 | 3.3781 |
| H | 1.3963 | 2.9503 | -3.7671 |
| H | 3.7497 | 0.1936 | 3.7671 |
| C | 0.9711 | 3.8464 | -3.2992 |
| C | 3.3245 | 1.0898 | 3.2992 |
| O | 0.6460 | 2.6491 | -0.8231 |
| O | 2.9995 | 5.4058 | 0.8231 |
| O | 0.6459 | 5.0429 | -0.8229 |
| O | 2.9993 | 2.2862 | 0.8229 |
| O | 2.9250 | 3.8461 | -1.4274 |
| O | 0.5715 | 1.0894 | 1.4274 |
| O | 2.5717 | 1.0893 | -1.6026 |
| O | 0.2183 | 3.8460 | 1.6026 |

### D. $Cl_2Hf_2$

| | |
|---|---|
| **Formula**: | $Cl_2Hf_2$ |
| **Database ID**: | MPDS S541493 |
| **3D Spacegroup**: | 166 ($R\bar{3}m$) |
| **Inversion symmetry**: | YES |
| **Direct Gap [meV]**: | 264.5 |
| **Indirect gap [meV]**: | -165.5 |
| **Binding energy DF2-C09 [meV/Å$^2$]**: | 14.8 |

TABLE VIII: Structural parameters

| | X[Å] | Y[Å] | Z[Å] |
|---|---|---|---|
| **a1** | 1.6926 | -2.9316 | 0.0000 |
| **a2** | 1.6926 | 2.9316 | 0.0000 |
| **a3** | 0.0000 | 0.0000 | 23.5715 |
| Hf | 0.0000 | 0.9772 | -1.1509 |
| Cl | 1.6926 | 0.0000 | -2.9083 |
| Hf | 0.0000 | -0.9772 | 1.1509 |
| Cl | 1.6926 | 0.0000 | 2.9083 |

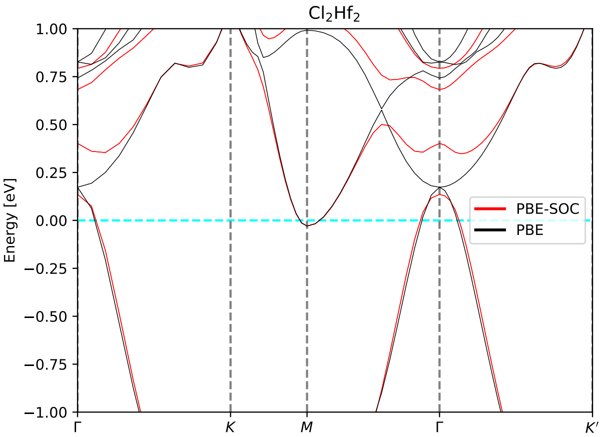


FIG. 19: DFT band structure with (red) and without (black) spin-orbit coupling.

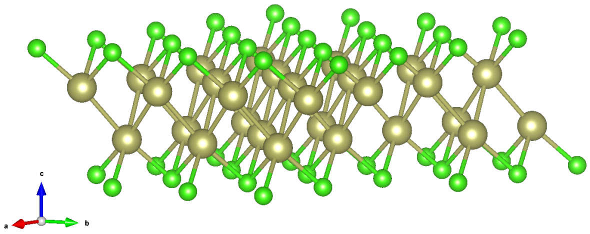

FIG. 20: Bird-eye view of the crystal structure.

### E. $Fe_4O_6$

| | |
|---|---|
| **Formula**: | $Fe_4O_6$ |
| **Database ID**: | MPDS S1024644 |
| **3D Spacegroup**: | 63 (Cmcm) |
| **Inversion symmetry**: | YES |
| **Direct Gap [meV]**: | 17.4 |
| **Indirect gap [meV]**: | -20.9 |
| **Binding energy DF2-C09 [meV/Å$^2$]**: | 6.4 |

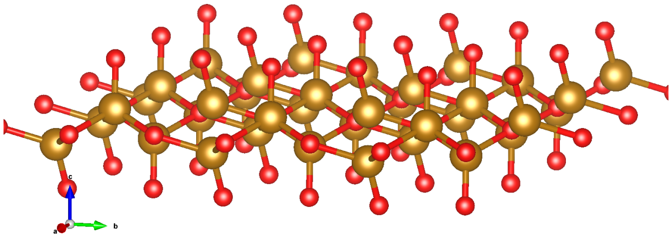

FIG. 23: Bird-eye view of the crystal structure.

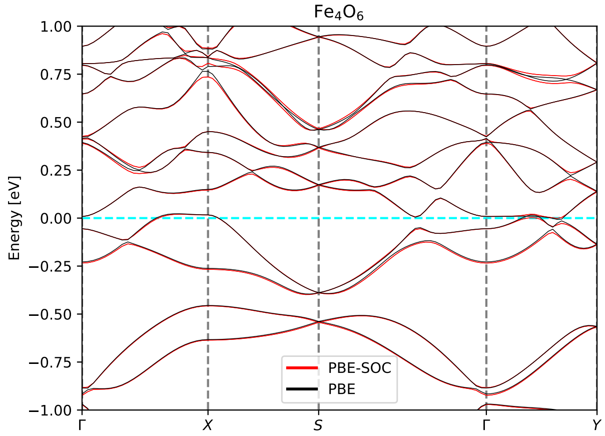


FIG. 21: DFT band structure with (red) and without (black) spin-orbit coupling.

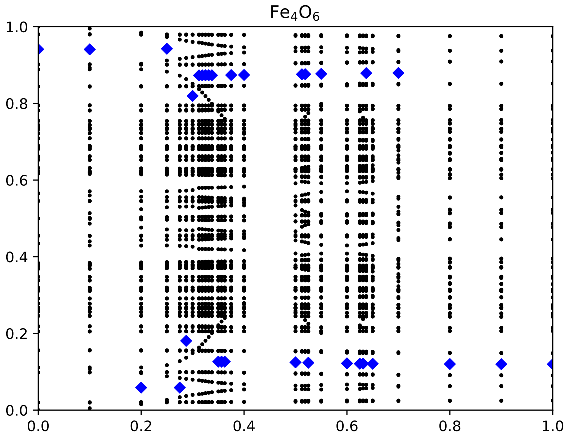


FIG. 22: Evolution of the HWCC (black dots) and largest gap positions (blue squares) across the Brillouin zone.

TABLE IX: Structural parameters

| | X[Å] | Y[Å] | Z[Å] |
|---|---|---|---|
| **a1** | 0.0000 | -4.4401 | 0.0000 |
| **a2** | 5.0537 | 0.0000 | 0.0000 |
| **a3** | 0.0000 | 0.0000 | 20.2558 |
| Fe | 4.7399 | -1.2408 | 0.6055 |
| Fe | 2.2130 | -3.1992 | 0.6055 |
| O | 4.5735 | -1.8252 | 2.0631 |
| O | 2.0466 | -2.6149 | 2.0631 |
| Fe | 2.8407 | -1.2408 | -0.6055 |
| Fe | 0.3138 | -3.1992 | -0.6055 |
| O | 3.0071 | -1.8252 | -2.0631 |
| O | 0.4802 | -2.6149 | -2.0631 |
| O | 1.2634 | -0.3507 | 0.0000 |
| O | 3.7903 | -4.0893 | 0.0000 |

### F. $I_4Mo_2S_4$

| | |
|---|---|
| **Formula**: | $I_4Mo_2S_4$ |
| **Database ID**: | MPDS S376458 |
| **3D Spacegroup**: | 12 (C2/m) |
| **Inversion symmetry**: | YES |
| **Direct Gap [meV]**: | 47.0 |
| **Indirect gap [meV]**: | -116.5 |
| **Binding energy DF2-C09 [meV/Å$^2$]**: | 14.4 |

TABLE X: Structural parameters

| | X[Å] | Y[Å] | Z[Å] |
|---|---|---|---|
| **a1** | 3.6777 | -5.7905 | 0.0000 |
| **a2** | 3.6777 | 5.7905 | 0.0000 |
| **a3** | 0.0000 | 0.0000 | 19.9256 |
| I | -1.1916 | 2.3325 | 1.5943 |
| I | -1.1916 | 9.2484 | 1.5943 |
| Mo | 0.0000 | 4.3943 | 0.0000 |
| Mo | 0.0000 | 7.1866 | 0.0000 |
| I | -2.4861 | 8.1229 | -1.5943 |
| I | -2.4861 | 3.4580 | -1.5943 |
| S | -1.7536 | 5.7905 | 0.9604 |
| S | 0.0294 | 5.7905 | 1.9731 |
| S | 1.7536 | 5.7905 | -0.9604 |
| S | -0.0294 | 5.7905 | -1.9731 |

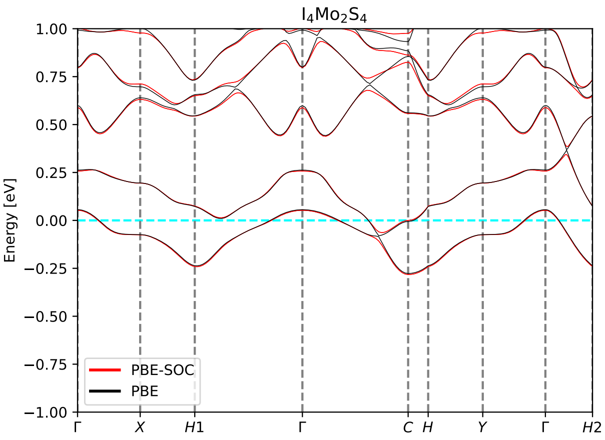


FIG. 24: DFT band structure with (red) and without (black) spin-orbit coupling.

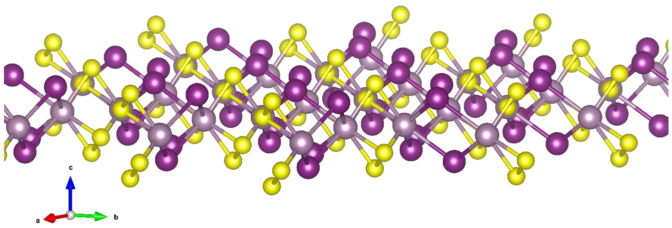

FIG. 25: Bird-eye view of the crystal structure.

### G. $Mo_2O_{17}Ta_2$

| | |
|---|---|
| **Formula**: | $Mo_2O_{17}Ta_2$ |
| **Database ID**: | ICSD 247163 |
| **3D Spacegroup**: | 166 ($R\bar{3}m$) |
| **Inversion symmetry**: | NO |
| **Direct Gap [meV]**: | 16.9 |
| **Indirect gap [meV]**: | -36.3 |
| **Binding energy DF2-C09 [meV/Å$^2$]**: | 10.0 |

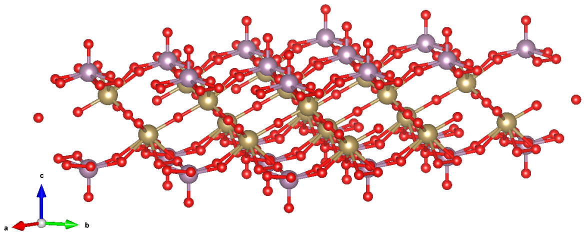

FIG. 28: Bird-eye view of the crystal structure.

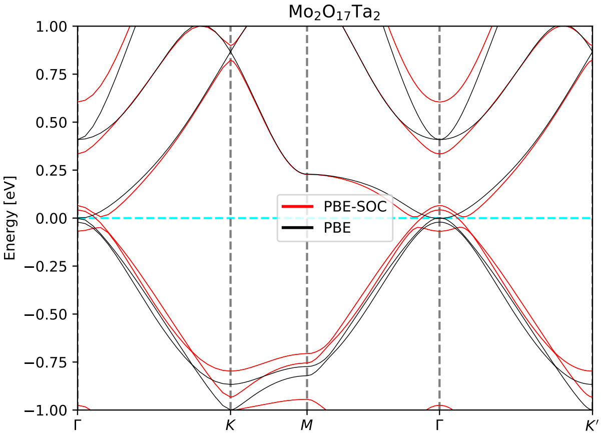


FIG. 26: DFT band structure with (red) and without (black) spin-orbit coupling.

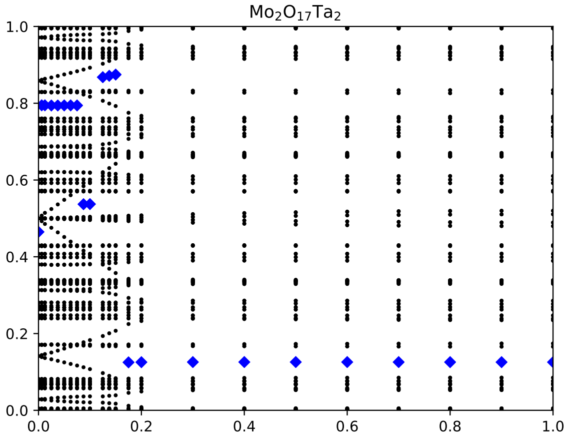


FIG. 27: Evolution of the HWCC (black dots) and largest gap positions (blue squares) across the Brillouin zone.

TABLE XI: Structural parameters

| | X[Å] | Y[Å] | Z[Å] |
|---|---|---|---|
| **a1** | 3.0670 | -5.3122 | 0.0000 |
| **a2** | 3.0670 | 5.3122 | 0.0000 |
| **a3** | 0.0000 | 0.0000 | 29.7696 |
| Ta | 1.5335 | -0.8854 | 0.9405 |
| Mo | 1.5335 | 2.6561 | 2.8350 |
| O | 1.5335 | 2.6561 | 4.5001 |
| O | 3.3929 | -1.1177 | 2.3804 |
| O | 0.8050 | 0.8411 | 2.3804 |
| O | -0.3259 | -1.1178 | 2.3804 |
| O | 2.2620 | 0.8411 | 2.3804 |
| O | 0.4025 | -2.3795 | 2.3804 |
| O | 2.6645 | -2.3795 | 2.3804 |
| Ta | 4.6005 | 0.8854 | -0.9405 |
| Mo | 1.5335 | 2.6561 | -2.8350 |
| O | 1.5335 | 2.6561 | -4.5001 |
| O | 0.0000 | 0.0000 | 0.0000 |
| O | 1.5335 | -2.6561 | 0.0000 |
| O | 3.0670 | 0.0000 | 0.0000 |
| O | -0.4025 | 2.3795 | -2.3804 |
| O | 2.7411 | 1.1178 | -2.3804 |
| O | 2.2620 | 4.4711 | -2.3804 |
| O | 0.3259 | 1.1178 | -2.3804 |
| O | 3.4695 | 2.3795 | -2.3804 |
| O | 0.8050 | 4.4711 | -2.3804 |

* davide.grassano@epfl.ch

[1] K. Momma and F. Izumi, Journal of applied crystallography **44**, 1272 (2011).
